# Supplementary material for: Systematic analysis reveals key microRNAs as diagnostic and prognostic factors in progressive stages of lung cancer
Source: arXiv:2201.05408 source file (2022-01-14)
Supplement: Supplementary file 1 [file Supplementary_Information.pdf]

Supplementary Information for

# Systematic analysis reveals key microRNAs as diagnostic and prognostic factors in progressive stages of lung cancer

Dietrich Kong, Ke Wang, Qiu-Ning Zhang, and Zhi-Tong Bing
Corresponding author: Zhi-Tong Bing

## Contents

**Supplementary Notes** **1**
Note 1: TNM stages . . . 1
Note 2: Cox proportional hazards model . . . 1
Note 3: Survival curves . . . 2
Note 4: Statistical analysis and P-value . . . 2

**Supplementary Figures** **3**
KEGG enrichment analysis of DE microRNAs . . . 3
Correlation between eigenvectors and microRNA expression . . . 4
The FC value and expressions of prognostic factors . . . 5
MicroRNAs that affect patient survival . . . 5

**Supplementary Tables** **7**
Number of patients and DE microRNAs . . . 7
Number of censored patients . . . 7
Cox regression model . . . 8
TNM Staging groupings . . . 9

# Supplementary Notes

## Note 1: TNM stages

The International Association for the Study of Lung Cancer established the Lung Cancer Staging Project in 1998 and updated the Tumor-Node-Metastasis (TNM) classification system of malignant tumors [1], which formed the basis for classifying lung cancer into distinct stages. The current (seventh) edition classifies all histotypes of lung cancer after evaluation of the outcomes from an extensive worldwide database of patients.

TNM characterizes the size and location of the tumor, the location of cancer in the lymph nodes and to where the cancer has spread (Metastases). In particular, the letter "T" stands for primary tumor:

**"T1a"** – tumor size $\leq$ 2cm;
**"T1b"** – tumor size $> 2 \sim$ 3cm;
**"T2a"** – tumor size $> 3 \sim$ 5cm;
**"T2b"** – tumor size $> 5 \sim$ 7cm;
**"T3"** – tumor size $>$ 7cm and/or multiple tumor nodules in the same lobe;
**"T4"** – multiple tumor nodules (of any size) in the same lung but in a different lobe.

The letter "N" denotes the spread of the cancer to nearby lymph nodes:

**"N0"** – no regional lymph node metastasis;
**"N1"** – metastasis in ipsilateral peribronchial and/or ipsilateral hilar lymph nodes as well as intrapulmonary nodes including involvement by direct extension;
**"N2"** – metastasis in ipsilateral mediastinal and/or subcarinal lymph node(s);
**"N3"** – metastasis in contralateral mediastinal, contralateral hilar, ipsilateral or contralateral scalene, or supraclavicular lymph node(s).

The letter "M" describes distant metastasis:

**"M1a"** – malignant pleural or pericardial effusions and/or separate tumor nodules in the contralateral lung;

**"M2b"** – distant metastasis in extrathoracic organs.

Based on the TNM classification system described above, we listed the stage groupings for non-small-cell lung cancer in Supplementary Table 6. In order to retain sufficient data for statistical analysis in each LUAD stage, in our work, we combined stages Ia and Ib and label them as stage I, and did the same for stages II, III, and IV respectively.

## Note 2: Cox proportional hazards model

Cox proportional hazards model is a semiparametric regression model [2], Cox model can handle multifactor survival data and its defined hazard $h(t, X)$ is used as the dependent variable:

$$\mathbf{h}(\mathbf{t}, \mathbf{X}) = h_0(t) \exp(\beta_1 \star x_1 + \beta_2 \star x_2 + \cdots + \beta_p \star x_p) \tag{1}$$

$t$ is survival time, $x$ represents covariates related to survival time, where **h(t,X)** is the risk of covariate $x$ at time $t$ function.

The partial regression coefficient $\beta_p$ in the risk function 1 is the change in the degree of risk caused by each additional unit of the covariate $X_p$ when other covariates remain unchanged. Hazard Ratios (HR) is defined as:

$$HR = exp(\beta) \tag{2}$$

According to the formula 2:

- If $\beta > 0$, $HR > 0$, the greater the value of each $X$, the greater the value of $h(t, X)$, that is, the value of $X$ Risk factors.

- If $\beta = 0$ and $HR = 1$, the value of each $X$ has no effect on the value of HR, that is, $X$ is an irrelevant factor.
- If $\beta < 0$, $HR < 0$, the larger the value of each $X$, the smaller the value of $h(t, X)$, that is, $X$ is Protection factors.

## Note 3: Survival curves

Corroborating the results in Fig. 5 in the main text, we calculated the microRNA-based survival curves [3] of LUAD patients at each stage. As described in the main text, microRNAs hsa-mir-153-2, hsa-mir-424, hsa-mir-323b, and hsa-mir-19b-1 affect the survival of LUAD patients in middle- and later-stage respectively. Further support for this finding was presented in Supplementary Fig. 4, which showed that microRNAs hsa-mir-153-2 (P=0.047) and hsa-mir-424 (P=0.02) have an effect on the survival of LUAD patients in all stages. Additionally, P-values in Kaplan-Meier survival curves of hsa-mir-153-2 and hsa-mir-424 are 0.028 and 0.056 respectively.

## Note 4: Statistical analysis and P-value

We have used statistical analysis involving hypothesis testing to calculate P-values.

- In our data processing, microRNAs were processed through differentially expressed analysis, where the basic statistics for significance assessment are the moderated t-statistic [4], which is computed for each comparison. This has the same interpretation as ordinary t-statistics, except that the standard error has been moderated between genes, i.e., squeezed towards a common value, using a simple Bayesian model. This has the effect of borrowing information from the ensemble of genes to enhance inference about individual gene. Moderated t-statistics lead to P-values in the same way that ordinary t-statistics do except that the degrees of freedom are increased, reflecting the greater reliability associated with the smoothed standard error.

# References


[1] Goldstraw, P. *et al.* The IASLC Lung Cancer Staging Project: proposals for the revision of the TNM stage groupings in the forthcoming (seventh) edition of the TNM Classification of malignant tumours. *J. Thoracic Oncol.* **2**, 706–714 (2007).

[2] Cox, D. R. Regression models and life-tables. *Journal of the Royal Statistical Society: Series B (Methodological)* **34**, 187–202 (1972).

[3] Kleinbaum, D. G. & Klein, M. *Survival analysis*, vol. 3 (Springer, 2010).

[4] Phipson, B., Lee, S., Majewski, I. J., Alexander, W. S. & Smyth, G. K. Robust hyperparameter estimation protects against hypervariable genes and improves power to detect differential expression. *Ann. Appl. Stat.* **10**, 946 (2016).

# Supplementary Figures

## KEGG enrichment analysis of DE microRNAs

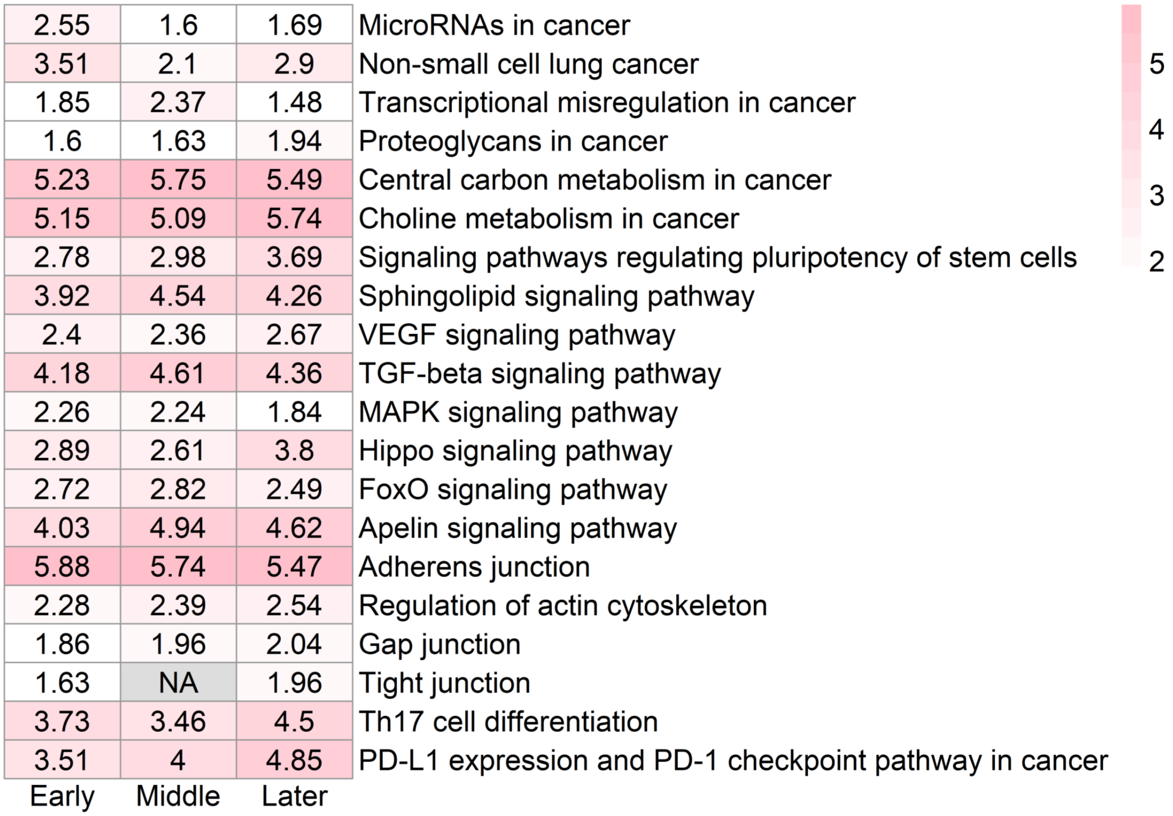


**Supplementary Figure 1. KEGG enrichment analysis of DE microRNAs associated with three stages of LUAD**. The columns "early" to "later"showed the results of microRNAs in the three stages. The value of the heat map is $-\log_{10} P$ from the enrichment analysis. The P-value is calculated using the hypergeometric distribution test, results from KEGG enrichment analysis. It reveals that those microRNAs are closely related to the biological functions of the cancer pathway, signal translation, and immune pathway.

## Correlation between eigenvectors and microRNA expression

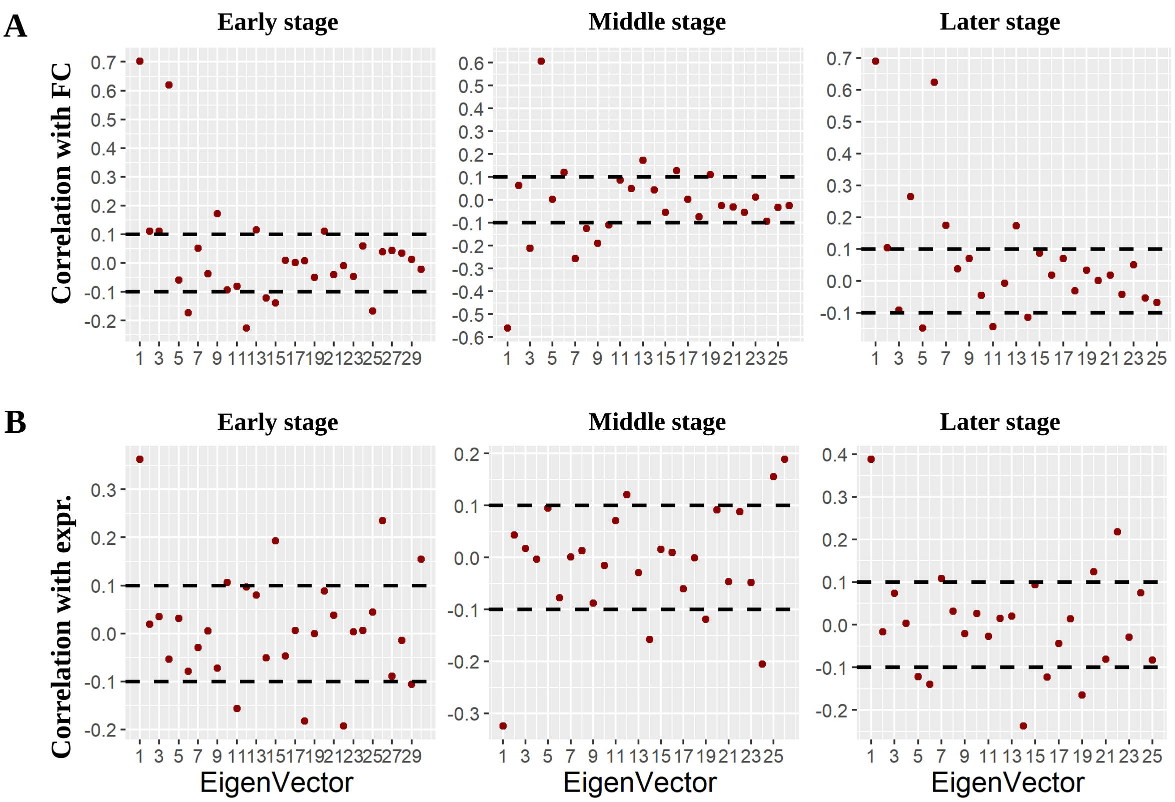


**Supplementary Figure 2. Correlation between eigenvectors and microRNA-expressed features**. The relationship between 30, 26, and 25 eigenvectors and A. gene expression or B. Fold-Change (FC) value from DE analysis in the early, middle, and later stages of LUAD. The Pearson correlation coefficients between eigenvector weight and RNA expression or FC value are within plus or minus 0.3, indicating that the eigenvectors are all to a great extent independent with microRNA expressed features, such as FC and expressions.

## The FC value and expressions of prognostic factors

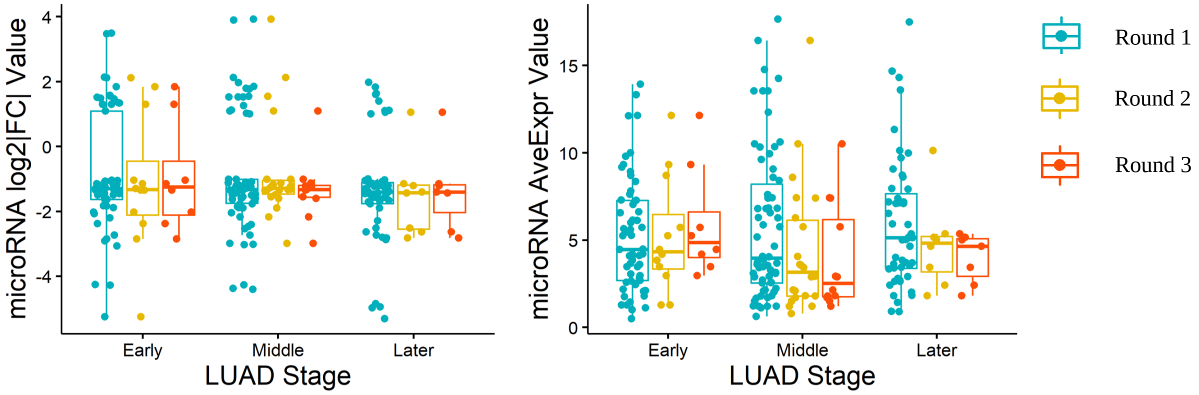


**Supplementary Figure 3. The FC value and expressions of microRNA with prognosis in three stages of LUAD**. In the three training rounds of the model, the log2|FC| value and average expression level of microRNA molecules used were shown in the two figures with blue, yellow, and red dots, respectively. The distribution of the molecular FC values in the same round had a high similarity, and that of the average expression also showed the same characteristic. In addition, at the same stage, both log2|FC| value and average expression of microRNA revealed an analogical distribution pattern in the different rounds, indicating that the factors obtained after each model screening were independent variables from their expression characteristics.

## MicroRNAs that affect patient survival

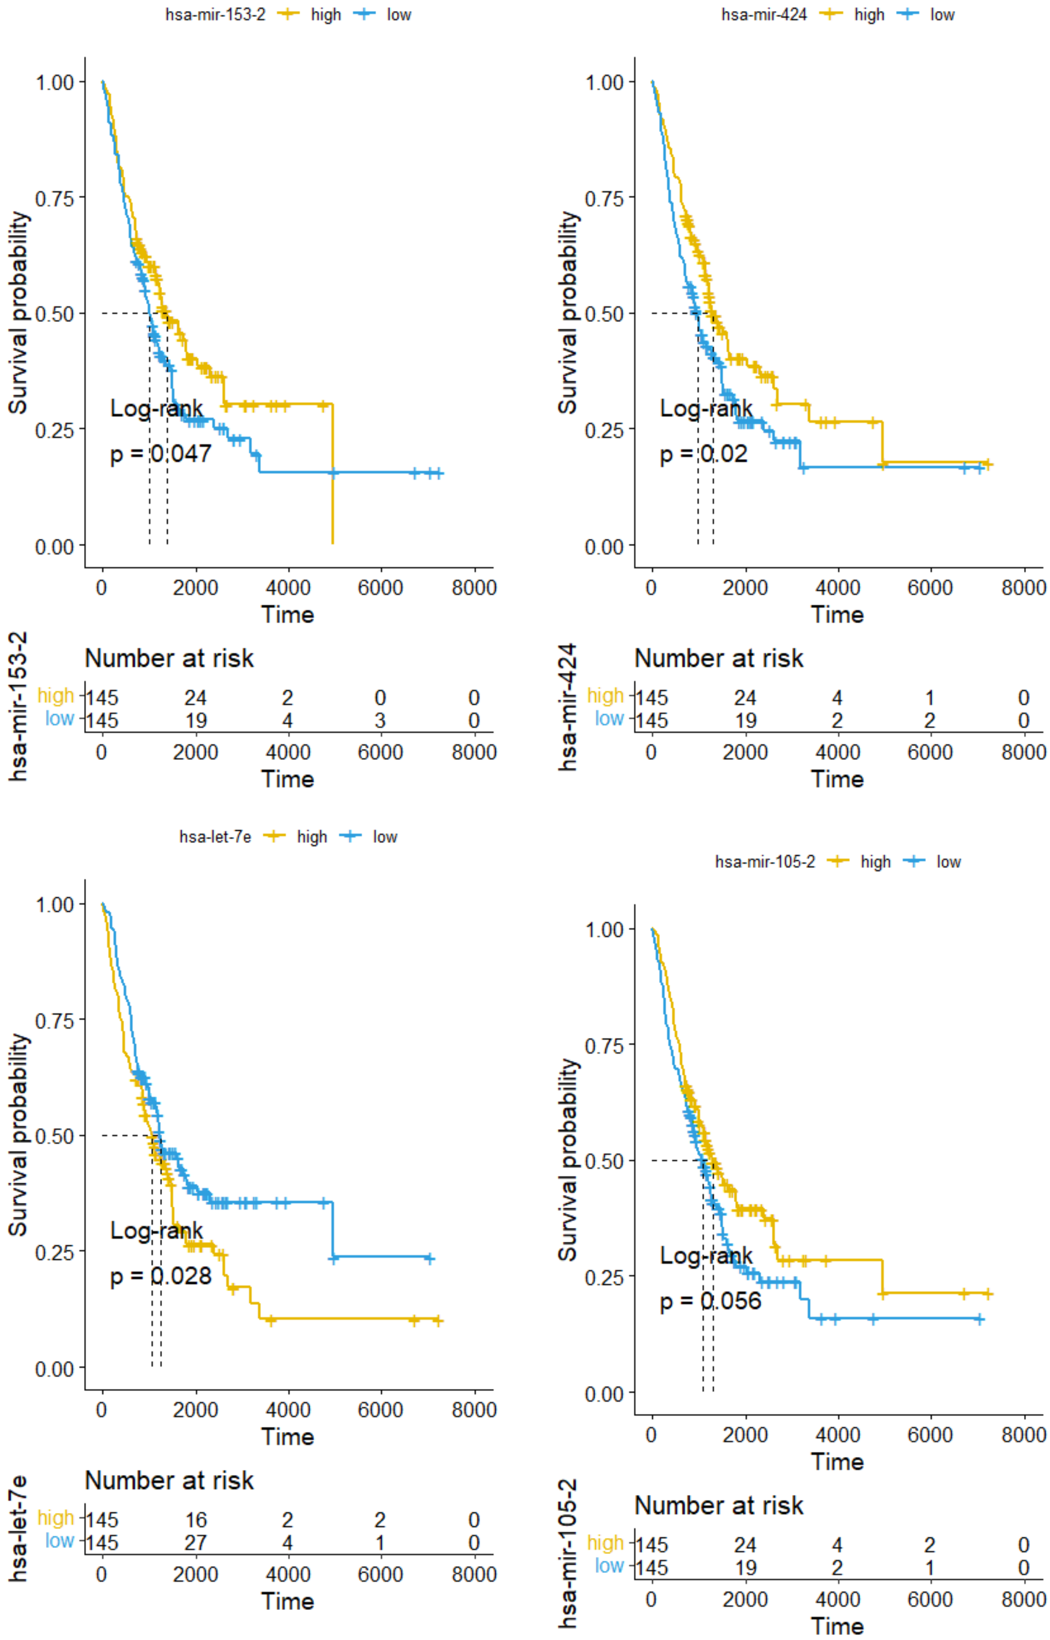


**Supplementary Figure 4. MicroRNAs that affect patient survival in all stages of LUAD**. Survival curves of the key microRNAs from Kaplan-Meier analysis and four microRNAs of prognostic factors have a significant influence on patient survival in all stages of LUAD. Log-rank tests were used to analyze the Kaplan-Meier survival curve.

# Supplementary Tables

## Number of patients and DE microRNAs

**Supplementary Table 1.** The row denoted as “Samples inter. with survi.” represents the numbers of samples that have matched the microRNA expression with clinical survival data of LUAD. The row “Final Samples” gives the number of samples in prognosis analysis.

Distribution of clinical samples and the number of DE microRNAs in LUAD

<table>
<tr><th rowspan="2"></th><th rowspan="2">Normal</th><th>Early stage</th><th>Middle stage</th><th colspan="2">Later stage<br>(stage III-IV)</th><th rowspan="2">Total</th></tr>
<tr><th>stage I</th><th>stage II</th><th>stage III</th><th>stage IV</th></tr>
<tr><td>Samples</td><td>46</td><td>279</td><td>122</td><td>84</td><td>24</td><td>555</td></tr>
<tr><td rowspan="2">Samples inter.<br>with survi.</td><td rowspan="2">46</td><td rowspan="2">273</td><td rowspan="2">120</td><td>80</td><td>23</td><td rowspan="2">542</td></tr>
<tr><td colspan="2">103</td></tr>
<tr><td>Final Samples</td><td>46</td><td>126</td><td>87</td><td colspan="2">77</td><td>336</td></tr>
<tr><td rowspan="2">DE microRNA</td><td rowspan="2">\</td><td rowspan="2">127</td><td rowspan="2">130</td><td>134</td><td>124</td><td rowspan="2">124</td></tr>
<tr><td colspan="2">131</td></tr>
</table>

## Number of censored patients

**Supplementary Table 2.** In order to balance the two types of survival data as much as possible, K years were taken as the classification criteria in the three stages respectively. Those who were followed up “censored” or lived “certain” for longer than the criteria belonged to “survival year > K”, otherwise the dead “certain” were marked as “survival year < K” and the data of the living were discarded.

Patients division based on survival data in three satges of LUAD

<table>
<tr><th rowspan="2"></th><th rowspan="2">Classification<br>Criteria: K Year</th><th>Survival year <K</th><th colspan="2">Survival year >=K</th><th rowspan="2">Total</th></tr>
<tr><th>Certain</th><th>Certain</th><th>Censored</th></tr>
<tr><td rowspan="2">Early Stage</td><td rowspan="2">3</td><td rowspan="2">40</td><td>26</td><td>60</td><td rowspan="2">126</td></tr>
<tr><td colspan="2">86</td></tr>
<tr><td rowspan="2">Middle Stage</td><td rowspan="2">2</td><td rowspan="2">32</td><td>26</td><td>34</td><td rowspan="2">87</td></tr>
<tr><td colspan="2">55</td></tr>
<tr><td rowspan="2">Later Stage</td><td rowspan="2">2</td><td rowspan="2">43</td><td>26</td><td>16</td><td rowspan="2">77</td></tr>
<tr><td colspan="2">34</td></tr>
</table>

## Cox regression model

**Supplementary Table 3.** According to the Cox proportional regression model 1, the eigenvectors of the first, middle, and later stages of LUAD were compared with gender and age for multivariate analysis. Calculated using the "survival" package of R software, and selected thresholds $p < 0.05$(maximum likelihood ratio test) and $|HR - 1| > 0.1$. The results were shown below

Using Cox regression model to analyse the eigenvectors and clinical features.

| | Item | P-value | HR($\beta$) | $Coef$ | Low(95% CI) | Up(95% CI) |
|---|---|---|---|---|---|---|
| Early Stage | V13 | 0.0027 | 1.194 | 0.1773 | 1.0636 | 1.3403 |
| | V18 | 0.0456 | 1.1521 | 0.1416 | 1.0028 | 1.3236 |
| | V27 | 0.0139 | 1.2759 | 0.2437 | 1.0508 | 1.5492 |
| | V30 | 0.0479 | 0.8167 | -0.203 | 0.6682 | 0.9982 |
| | sex | 0.8372 | 1.0537 | 0.0523 | 0.6401 | 1.7345 |
| | age | 0.5283 | 0.9916 | -0.008 | 0.966 | 1.0179 |
| Middle Stage | sex | 0.8372 | 1.0537 | 0.0523 | 0.6401 | 1.7345 |
| | age | 0.5283 | 0.9916 | -0.008 | 0.966 | 1.0179 |
| Later Stage | V8 | 0.0452 | 1.1024 | 0.0975 | 1.0021 | 1.2129 |
| | V13 | 0.032 | 1.1247 | 0.1175 | 1.0102 | 1.2522 |
| | V20 | 0.0037 | 0.8055 | -0.216 | 0.6959 | 0.9322 |
| | V25 | 0.008 | 1.2426 | 0.2172 | 1.0583 | 1.4589 |
| | sex | 0.7391 | 1.0908 | 0.0869 | 0.654 | 1.8194 |
| | age | 0.7127 | 0.9959 | -0.004 | 0.9745 | 1.0178 |

## TNM Staging groupings

**Supplementary Table 4.** Staging groupings for non-small-cell lung cancer.

| | Tumour (T) | Node (N) | Metastasis (M) |
|---|---|---|---|
| Ia | T1a or T1b | N0 | M0 |
| Ib | T2a | N0 | M0 |
| IIa | T1a or T1b | N1 | M0 |
| | T2a | N1 | M0 |
| | T2b | N0 | M0 |
| IIb | T2b | N1 | M0 |
| | T3 | N0 | M0 |
| IIIa | T1 or T2 | N2 | M0 |
| | T3 | N1 or N2 | M0 |
| | T4 | N0 or N1 | M0 |
| IIIb | T4 | N2 | M0 |
| | any T | N3 | M0 |
| IV | any T | any N | M1a |
| | any T | any N | M1b |
